# Supplementary material for: Continual Learning: Forget-free Winning Subnetworks for Video Representations
Source: arXiv:2312.11973 source file (2024-12-19)
Supplement: Supplementary file 1 [file datasets.tex]

\begin{table}[!ht]
\small
\centering
\vspace{-0.05in}
\caption{\small \textbf{Task-agnositic Incremental Learning (TaIL)}, Statistics on three datasets}
\resizebox{0.5\textwidth}{!}{
\begin{tabular}{lccc}
\toprule 

%\multicolumn{1}{c}{\multirow{2}{*}{\textbf{Method}}} & \multicolumn{8}{c}{\textbf{Video Sessions}} & \multirow{2}{*}{\thead{\textbf{Avg. PSNR / } \\ \textbf{BWT}}} \\ % & \multirow{2}{*}{\textbf{CAP}}  \\

%\cline{2-9}
& \textbf{Seq-CIFAR10} & \textbf{Seq-CIFAR100} & \textbf{Seq-TinyImageNet}  \\ \midrule 
\midrule

Task Number & 5 & 5 & 10 \\
Input Size & $3 \times 3 \times 32$ & $3 \times 32 \times 32$ & $3 \times 64 \times 64$ \\
Classes per Task & 5 & 20 & 20 \\
Training Samples & 10,000 & 10,000 & 10,000 \\
Test Samples & 1,000 & 1,000 & 1,000 \\

\bottomrule
\end{tabular}
}
\label{table:cil_dataset}
\vspace{-0.1in}
\end{table}
