# Supplementary material for: Continual Learning: Forget-free Winning Subnetworks for Video Representations
Source: arXiv:2312.11973 source file (2024-12-19)
Supplement: Supplementary file 3 [file reviewer01_r1.tex]

\subsection{Dear Revewer1}
Thank the reviewer for constructive suggestions regarding the main novelty. Based on the reviewer's concrete feedbacks, we have further strengthened our contributions to continual learning. We have summarised as follows:


\begin{itemize}[leftmargin=*]
        \item \textcolor{blue}{(Performances of WSN on FSCIL): As the reviewer’s suggestion, we have included WSN’s performance on three FSCIL scenarios, as presented in the main script of Tables 3, 4, and 5. The results show that SoftNet (+ FSO) consistently outperforms WSN’s baseline across all three benchmark datasets. This ablation study further highlights the effectiveness of FSO in addressing two challenges: mitigating the abstracted representation issues inherent in ResNet structures and reducing overfitting in FSCIL scenarios.}

    \item \textcolor{blue}{(Why not use SoftNet across all experiments instead of WSN? And why is WSN necessary?): We have prepared the following three responses regarding the question of not using SoftNet in all continual learning scenarios (TIL, TaIL, VIL, and FSCIL):}
    
    \begin{itemize}
        \item \textcolor{blue}{Comparative sparse solutions across continual Learning scenarios:} WSN and SoftNet provide comparable sparse solutions for TIL, TaIL, and VIL. In TIL and TaIL, session datasets are separated by distinct image category subsets, while in VIL, sessions are defined by independent video clips. For these scenarios, SoftNet’s major ticket (m=1) is identical to WSN’s ($m=1$), ensuring parameter-efficient sparse solutions superior to dense networks. In contrast, FSCIL presents a unique challenge of imbalanced session datasets: the base session ($s=1$) contains abundant samples, while subsequent sessions ($s>1$) provide a few-shot (e.g., 5-way 5-shot) to models. SoftNet addresses this severe imbalance by updating only minor tickets ($m<1$), effectively mitigating overfitting issues significantly more pronounced in FSCIL than in TIL, TaIL, and VIL. To demonstrate SoftNet’s effectiveness in FSCIL, we have added WSN baselines to our evaluation, as shown in the main script of Tables 3, 4, and 5.
        
        \item \textcolor{blue}{Effectiveness of Minor Tickets ($m<1$):} Additionally, to further explore SoftNet’s advantages and investigate the effect of minor tickets ($m<1$), particularly in TIL, we have analyzed the differences between WSN and SoftNet (see \Cref{fig:conf_soft_wsn_cifar100}). Observations reveal that SoftNet’s small perturbed tickets ($m<1$) enhance forward transferability through the adaptive reuse of parameters ($m=1$) guided by session sample similarity. The adaptive reusability of parameters depends on sample or task similarity, which we have already analyzed from the ICML2022 paper. Therefore, this is not the main focus of this work.
        
        \item \textcolor{blue}{(Main contribution in this work) Addressing representation challenges:} The primary goal of our work is to address two key challenges using FSO: (1) abstract representations: Loss of global image structures in higher layers (e.g., ResNets) across TIL, TaIL, CIL, and FSCIL and (2) lack of representation power in video-centric scenarios, i.e., VIL. Our novel FSO structures with ResNets and NeRVs are specifically designed to tackle these challenges. Extensive experiments demonstrate that our FSO effectively complements these representation issues across the WSN, SoftNet, and NeRVs structure.

        \item \textcolor{blue}{In conclusion, parameter-efficient sparse solutions like WSN are crucial for mitigating overfitting in over-parameterized dense networks in continual learning scenarios. As a variant of WSN, SoftNet is uniquely tailored to address the severe overfitting caused by imbalanced sequential session datasets in FSCIL. We hope the reviewer understands that our work highlights the representation challenges inherent in ResNets and NeRVs within the paper's page constraints and presents solutions through FSO structures.}
    \end{itemize}

    \item \textcolor{blue}{(Theoretical Analysis Structure): To enhance readers' understanding of our work, specifically the characteristics of WSN and SoftNet, we have refined the supplementary theoretical section. This revision introduces one foundational assumption and two essential components (Lemmas), forming the basis for a rigorous theoretical deduction.}

    \item \textcolor{black}{To address the reviewer’s concerns about the approach being a simple combination of three papers, we have provided additional explanations highlighting how we integrate various continual learning scenarios through challenging aspects and the insightful novelty of FSO.}

    \item \textcolor{black}{Regarding the new structure formed by combining WSN, SoftNet, and FSO, we have thoroughly explored all variations of WSN using FSO across different tasks, including classification (TIL, TaIL, FSCIL) and video representation learning (VIL).}

    \item \textcolor{black}{Originally, SoftNet was proposed to minimize catastrophic forgetting (CF) and mitigate overfitting issues in Few-Shot Class-Incremental Learning (FSCIL). A convergence theory was proposed to explain the differences between WSN and SoftNet. In this work, we have formulated a convergence theory to illustrate the relationship between WSN and SoftNet with FSO, which achieves a more global flat minima compared to DenseNet. Furthermore, we demonstrate the flatness of subnetworks through a 3D loss landscape, SoftNet's forward capability, and the Transfer Matrix in TIL to support the proposed theory.}






    \item To address the reviewer’s concerns about the approach being a simple combination of three papers, we have provided additional explanations highlighting how we integrate various continual learning scenarios through challenging aspects and the insightful novelty of FSO.

    \item Regarding the new structure formed by combining WSN, SoftNet, and FSO, we have thoroughly explored all variations of WSN using FSO across different tasks, including classification (TIL, TaIL, FSCIL) and video representation learning (VIL).

    \item Originally, SoftNet was proposed to minimize catastrophic forgetting (CF) and mitigate overfitting issues in Few-Shot Class-Incremental Learning (FSCIL). A convergence theory was proposed to explain the differences between WSN and SoftNet. In this work, we have formulated a convergence theory to illustrate the relationship between WSN and SoftNet with FSO, which achieves a more global flat minima compared to DenseNet. Furthermore, we demonstrate the flatness of subnetworks through a 3D loss landscape, SoftNet's forward capability, and the Transfer Matrix in TIL to support the proposed theory.
\end{itemize}

\subsection{Continual Learning Scenarios} 
The Catastrophic Forgetting (CF) is inevitable in all Continual Learning (CL) scenarios. Various approaches have been taken to alleviate the CF problem. Moreover, leveraged by abstracting representation, the CL model, i.e., ResNets, which performs sequential classifications such as TIL, TaIL, CIL, and FSCIL, has another challenging point: it loses the global structure of image instances at a high layer, leading to deteriorated classification performances. In this work, we refer to the issue as an \underline{(1) abstract representation}. In contrast, we observed a lack of representation power in VIL for sequential implicit neural representation learning, led by the conventional convolutional layer (NeRV). We refer to this issue as a \underline{(2) lack of representation power}. For the reader to understand the two challenges and the novel architecture-based points (\underline{FSO}), we briefly summarize the specific continual learning scenarios (TIL, TaIL, CIL, FSCIL, and VIL) as follows: \\

\noindent
\textbf{Task-Incremental Learning (TIL).} Each session is a separate classification problem. The session ID of instances is provided during training and testing, and the continual learner uses ConvNet or ResNet. TIL's model trains a sequence of sessions $s_1, s_2, \cdots, s_{|\mathcal{S}|}$, incrementally. Each session $s \in \mathcal{S}$ has a training dataset $\mathcal{D}_s = \{(\bm{x}_s^i, y_s^i)\}_{i=1}^{n_s}$ where $(\bm{x}_s^i, y_s^i) \in \mathcal{X} \times \mathcal{Y}_s$ and $\mathcal{Y}_s$ are disjoint and $\cup_{s=1}^{\mathcal{|S|}}\mathcal{Y}_s = \mathcal{Y}$. The objective is to learn $f_{\bm{\theta} \odot \bm{m}_s}: \mathcal{X} \times \mathcal{S} \rightarrow \mathcal{Y}$.  

\begin{itemize}[leftmargin=*]

\item (challenging points): CF, model size, \underline{(1) abstract representation}. 
\item (novelties): \underline{FSO}, WSN (previous work's novelty).

\end{itemize}


\noindent
\textbf{Task-agnositic Incremental Learning (TaIL).} The TaIL follows the same structure as TIL. However, the session ID of instances is \textbf{NOT} provided during training and testing, and the continual learner (ConvNet or ResNet) must infer the session ID in the testing, as stated in \Cref{sub_sec:opt_til}. The TaIL is the most challenging CL scenario.

\begin{itemize}[leftmargin=*]

\item (challenging points): CF, model size, session ID inference, \underline{(1) abstract representation}.
\item (novelties): \underline{FSO}, WSN (previous work's novelty).

\end{itemize}


\noindent
\textbf{Class-Incremental Learning (CIL).} The CIL process builds a single classifier for all sessions/classes learned so far. In training, the session ID of the instances is given to a continual learner (ConvNet or ResNet). However, in testing, an instance from any class may be presented for the model to classify. There is no prior session information on the test instance. CIL's model trains a sequence of sessions $s_1, s_2, \cdots, s_{|\mathcal{S}|}$, incrementally. Each session $s \in \mathcal{S}$ has a training dataset $\mathcal{D}_s = \{(\bm{x}_s^i, y_s^i)\}_{i=1}^{n_s}$ where $(\bm{x}_s^i, y_s^i) \in \mathcal{X}_s \times \mathcal{Y}_s$ and $\mathcal{Y}_s$ are disjoint and $\cup_{s=1}^{\mathcal{|S|}}\mathcal{Y}_s = \mathcal{Y}$. The objective is to learn $f_{\bm{\theta} \odot \bm{m}_s}: \mathcal{X} \times \mathcal{S} \rightarrow \mathcal{Y}$, where session ID $s$ is to be inferred in the testing time. 

\begin{itemize}[leftmargin=*]

\item (challenging points): CF, model size, session ID inference, \underline{(1) abstract representation}.
\item (novelties): \underline{FSO}, WSN (previous work's novelty).

\end{itemize}

\noindent
\textbf{Few-Shot Class-Incremental Learning (FSCIL).}
FSCIL follows the same structure as CIL. However, in new sessions ($s\geq 1$), only a \textbf{FEW} instances are given to the model, while abundant instances are in the base session ($s=1$). This makes it harder to train the CL model to avoid overfitting and alleviating CF simultaneously under the session ID that is not given in the test times.

\begin{itemize}[leftmargin=*]

\item (challenging points): CF, model size, session ID inference, \underline{(1) abstract representation}, \underline{overfitting}.
\item (novelties): \underline{FSO}, SoftNet (previous work's novelty to avoid overfitting).

\end{itemize}


\noindent
\textbf{Video-Incremental Learning (VIL).}
Each session is a separate video representation problem. The session ID of instances is provided during training and testing, and the continual learner uses NeRVs. VIL's model trains a sequence of sessions $s_1, s_2, \cdots, s_{|\mathcal{S}|}$, incrementally. Each session $s \in \mathcal{S}$ has a training dataset $\mathcal{D}_s = \{(\bm{x}_s^i, y_s^i)\}_{i=1}^{n_s}$ where $(\bm{x}_s^i, y_s^i) \in \mathcal{X} \times \mathcal{Y}_s$ and $\mathcal{Y}_s$ are disjoint and $\cup_{s=1}^{\mathcal{|S|}}\mathcal{Y}_s = \mathcal{Y}$. The objective is to learn $f_{\bm{\theta} \odot \bm{m}_s}: \mathcal{X} \times \mathcal{S} \rightarrow \mathcal{Y}$. 


\begin{itemize}[leftmargin=*]

\item (challenging points): \underline{(2) lack of representation power.}
\item (novelties): \underline{FSO}, WSN (previous work's novelty).

\end{itemize}


%\subsection{Concerns simply combine three papers}
%
%\textbf{Video Representations} 

\subsection{Variations of WSN through FSO}
Regarding the additional structures of WSN, SoftNet, and FSO, we could take various fusion methods such as element-wise summation and concatenations, however, these fusion methods are minor points in this work. We have investigated all variations of WSN using FSO in classification and video representations in this work. Through the inspections, we achieved the current state-of-the-art performances under continual learning scenarios. We summarize the two variations in terms of two types of architectures (ResNet, NeRVs). 

\begin{itemize}[leftmargin=*]

\item \underline{(1) abstract representation}: Through FSO, representations from the lower layer are fed to inputs at the higher layer (ResNets) to maintain global image representation, leading to the best performances in TIL, TaIL, CIL, and FSCIL.
\item \underline{(2) lack of representation power}: FSO captures global contextual representations to generate high-quality video images. We found the most parameter-efficient layer (f-NeRV3 with 8-bit qualitzation) of FSO since FSO's parameters increase at a higher layer (NeRVs).

\end{itemize}




% Since the authors are trying to connect all these three papers together, provide deeper insights on WSN and SoftNet than what is already presented in the published conference papers. Could WSN and SoftNet be unified under a common framework using FSO, or is there any general theoretical guarantee provided? Additionally, consider using FSO to structure more components beyond WSN and SoftNet.
\subsection{WSN and SoftNets through FSO}

We have unified various kinds of continual learning scenario (TIL, FSCIL, CIL, TaIL, and VIL) as well as Single Task Learning (STL, ImageNet-1K as shown in \Cref{table:imagnet1k} and \Cref{table:uvg8_stl}) through FSO, concretely. The remaining point is the relationship between WSN and SoftNet. The SoftNet, which incorporates minor winning tickets ($m < 1$), is a variant of WSN ($m \in \{0,1\}$) to alleviate the overfitting issues caused by few samples given in new session in the FSCIL scenario. Since the overfitting is not main issues in TIL, TaIL, CIL, and VIL, the effectiveness of SoftNet + FSO could be minor in those CL scenarios.

%As stated in previous paperwork~\cite{kang2022soft}, we would discuss WSN and SoftNet to remind the reviewer of this point.
However, we observed the powerful forward transfer ability of SoftNet in TIL where SoftNet was obtained by inducing small perturbation into zeros mask values. As shown in \Cref{tab:main_soft_til}, SoftNet obtained competitive performance with WSN and showed powerful forward transfer ability over WSN (see \Cref{fig:conf_soft_wsn_cifar100}). We could explain this result from the following convergence of WSN and SoftNet, stated in previous work~\cite{kang2022soft}: WSN and SoftNet have flatter minima than Dense Network, and small perturbed WSN (SoftNet) could predict unseen session instances in the flat minima. 

\noindent
\textbf{\textcolor{blue}{Convergences of WSN / SoftNet.}}
We hypothesize that fine-tuning SoftNet on flatter minima mitigates overfitting in FSCIL more effectively than WSN or dense networks on sharper minima since SoftNet, operating in flatter minima, is less prone to converging to local minima. To analyze SoftNet's convergence behavior, we adopt the framework of Lipschitz-continuous objective gradients~\cite{boyd2004convex, bottou2018optimization}:
\begin{lemma} 
\textbf{\textcolor{blue}{(Lipschitz Continuity of Dense Networks)}}: Let $R:\mathbb{R}^d \rightarrow \mathbb{R}$ be the objective function of a dense network, which is continuously differentiable. Its gradient function  $\nabla R: \mathbb{R}^d \rightarrow \mathbb{R}^d$, Lipschitz continuous with constant $L > 0$, satisfying the inequality:
\begin{equation} 
\begin{split}
    ||\nabla R(\bm{\theta}) - \nabla R(\bm{\theta}')||_2 & \leq  L||\bm{\theta} - \bm{\theta}'||_2, \;\; \\ 
    & \text{ for } \forall \bm{\theta}, \bm{\theta}' \in \mathbb{R}^d.
\end{split} 
\label{eq:dense_lip}
\end{equation}
\label{lm:dense_lip}
\end{lemma}

\begin{lemma}
\textbf{\textcolor{blue}{(Lipschitz Continuity of Subnetworks)}}: For a subnetwork defined by a binary mask $\bm{m}$, the objective function $R(\bm{\theta} \odot \bm{m})$ satisfies a sparsity-aware Lipschitz continuity condition:

\begin{equation} 
\begin{split}
    || \nabla R(\bm{\theta} \odot \bm{m}) - \nabla R(\bm{\theta}' \odot \bm{m}) ||_2 &\leq  L || (\bm{\theta} - \bm{\theta}') \odot \bm{m} ||_2, \\ 
    & \text{ for } \forall \bm{\theta}, \bm{\theta}' \in \mathbb{R}^d.
\end{split}
\label{eq:subnet_lip}
\end{equation}

Additionally, using the effective mask size $||\bm{m}||_{eff} = ||\bm{m}||_1^2 / ||\bm{m}||_2^2$, the above Lipschitz continuity condition is refined as:

\begin{equation} 
\begin{split}
    || \nabla R(\bm{\theta} & \odot \bm{m}) - \nabla R(\bm{\theta}' \odot \bm{m}) ||_2   \\
    %& \leq L || (\bm{\theta} - \bm{\theta}') \odot \bm{m} ||_2   \\
    & < \frac{L}{||\bm{m}||_{eff}}||(\bm{\theta}-\bm{\theta}')\odot\bm{m}||_2
\end{split}
\label{eq:subnet_lip_tight}
\end{equation}

\label{lm:subnet_lip}
\end{lemma}

\begin{theorem}
\textbf{\textcolor{blue}{(Convergence Rate of Subnetworks vs. Dense Networks)}}:
Subnetworks achieve a faster convergence rate compared to dense networks due to their simpler loss landscapes. For dense networks: $R(\bm{\theta}) = \mathcal{O}(d)$ where $d=||\bm{\theta}||_2$ while subnetwork: $R(\bm{\theta} \odot \bm{m})=\mathcal{O}(1/||\bm{m}||_2)$~\cite{ye2020good}. Given $||\bm{m}||_2 \ll d$, we observe the following comparison:
$$
\frac{R(\bm{\theta}\odot \bm{m})}{R(\bm{\theta})} = \frac{\mathcal{O}(1/||\bm{m}||_2)}{\mathcal{O}(d)}
$$
This suggests that subnetworks can achieve a faster convergence rate, i.e., $R(\bm{\theta} \odot \bm{m}) \ll R(\bm{\theta})$ because their effective loss landscape is less complex, leading to more efficient gradient descent steps. Using \textbf{\textit{Lemmas A.1}} and \textbf{\textit{A.2}}, we further deduce:
\begin{equation}
\begin{split}
    \frac{|| \nabla R(\bm{\theta} \odot \bm{m}) - \nabla R(\bm{\theta}' \odot \bm{m}) ||_2}{|| (\bm{\theta} - \bm{\theta}')\odot\bm{m}||_2}  & \\
    \leq \frac{|| \nabla R(\bm{\theta}) - \nabla R(\bm{\theta}') ||_2}{||\bm{\theta}- \bm{\theta}'||_2} & \leq L.
\end{split}
\end{equation}
This implies that subnetworks, due to their sparsity, exhibit a flatter loss landscape, which promotes more stable and generalizable solutions. The smaller the value is, the flatter the solution (loss landscape) is. The equation is established from the relationship $R(\bm{\theta} \odot \bm{m}) \ll R^\ast(\bm{\theta})$, where $R^\ast(\bm{\theta})$ denotes the best possible loss achievable by convex combinations of all dense network's parameters despite $|| (\bm{\theta} - \bm{\theta}') \odot \bm{m} ||_2 < ||\bm{\theta} - \bm{\theta}'||_2$. 
\end{theorem}

\begin{theorem}
\textbf{\textcolor{blue}{(Comparison of WSN and SoftNet)}}:
Consider two subnetworks, characterized by masks $\bm{m}_{WSN}$ and $\bm{m}_{SoftNet}$, where $||\bm{m}_{WSN}||_2 < ||\bm{m}_{SoftNet}||_2$. if the corresponding losses are approximately equal, i.e., $|| R(\bm{\theta} \odot \bm{m}_{WSN})-R(\bm{\theta} \odot \bm{m}_{SoftNet})||_2 \simeq 0$, then the following inequality holds:
\begin{equation} 
\begin{split}
    & \frac{|| \nabla R(\bm{\theta} \odot \bm{m}_{WSN}) - \nabla R(\bm{\theta}' \odot \bm{m}_{WSN}) ||_2}{|| (\bm{\theta} - \bm{\theta}') \odot \bm{m}_{WSN} ||_2}  \\ 
    &~~ \geq \frac{|| \nabla R(\bm{\theta} \odot \bm{m}_{SoftNet}) - \nabla R(\bm{\theta}' \odot \bm{m}_{SoftNet}) ||_2}{|| (\bm{\theta} - \bm{\theta}') \odot \bm{m}_{SoftNet}||_2},
\end{split}
\end{equation}
Equality is achieved \textit{iff} $||\bm{m}_{WSN}||_2 = ||\bm{m}_{SoftNet}||_2$. Moreover, the effective mask size using \textbf{\textit{Lemma A.2}} refines the following bound:
$$
\frac{L}{||\bm{m}_{WSN}||_{eff}} > \frac{L}{||\bm{m}_{SoftNet}||_{eff}}.
$$
This suggests that smaller effective masks in subnetworks lead to sharper loss landscapes. These conclusions also holds for $WSN + FSO$ and $SoftNet + FSO$.
\end{theorem}
Figure \Cref{fig:main_plot_loss_lens} visualizes the loss landscapes of dense networks, WSN, and SoftNet. The results illustrate that subnetworks (WSN and SoftNet) achieve flatter global minima than dense networks, with SoftNet exhibiting the flattest loss landscape. These findings support the theoretical claims regarding improved stability and generalization through sparse networks, such as WSN and SoftNet.

\input{supples/materials/plot_hard_soft}

\input{supples/materials/table_til_wsn_softnet_v1}
\input{supples/materials/table_conf_wsn_soft}
\input{supples/materials/table_corr_wsn_soft}
