# Supplementary material for: Continual Learning: Forget-free Winning Subnetworks for Video Representations
Source: arXiv:2312.11973 source file (2024-12-19)
Supplement: Supplementary file 5 [file reviewer03_r1.tex]

\subsection{Dear Reviewer3}

Thank the reviewer for constructive suggestions to strengthen our contributions to continual learning. 
